# Supplementary material for: Automated threshold selection and associated inference uncertainty for univariate extremes
Source: arXiv:2310.17999 source file (2024-10-29)

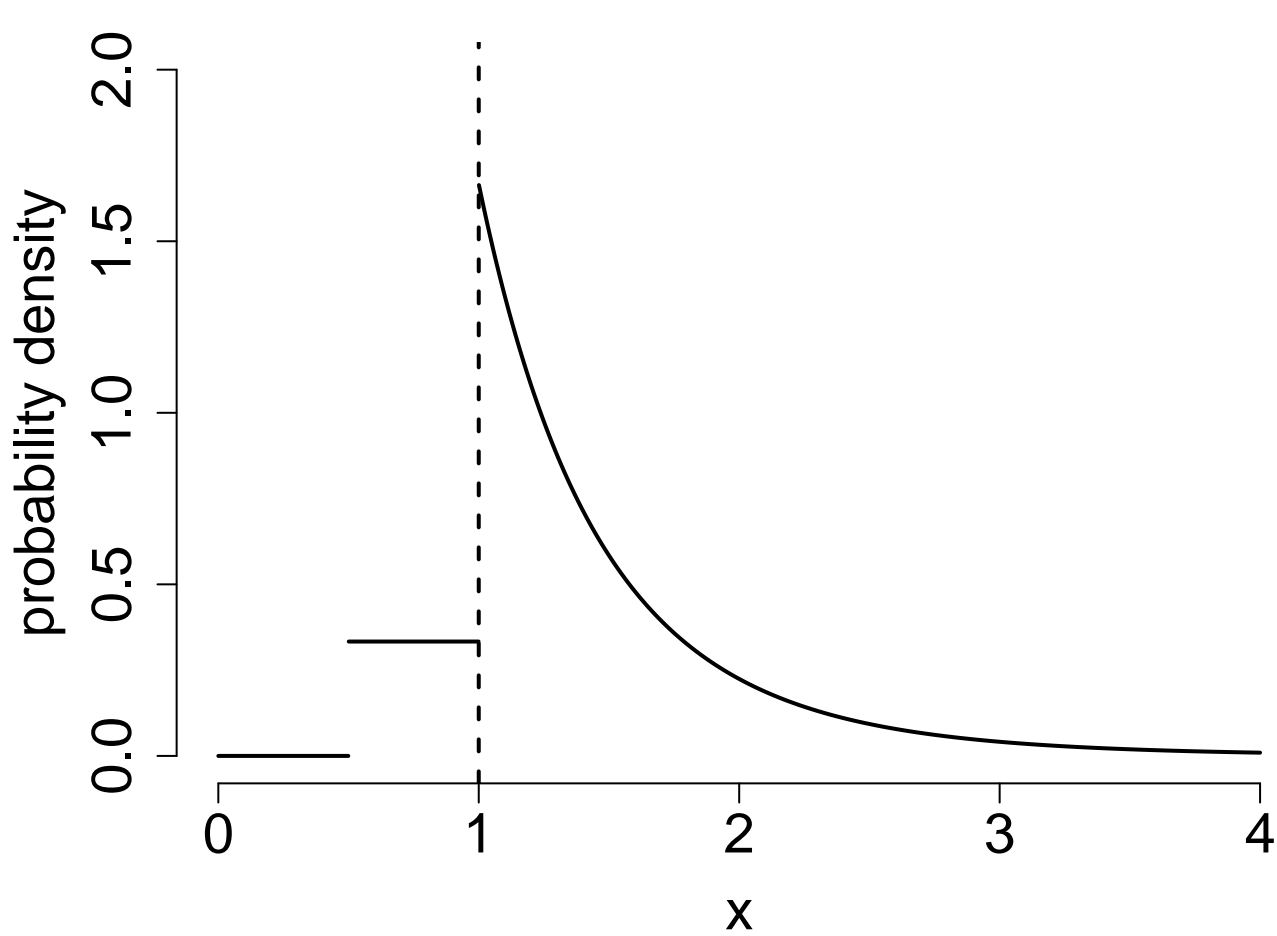

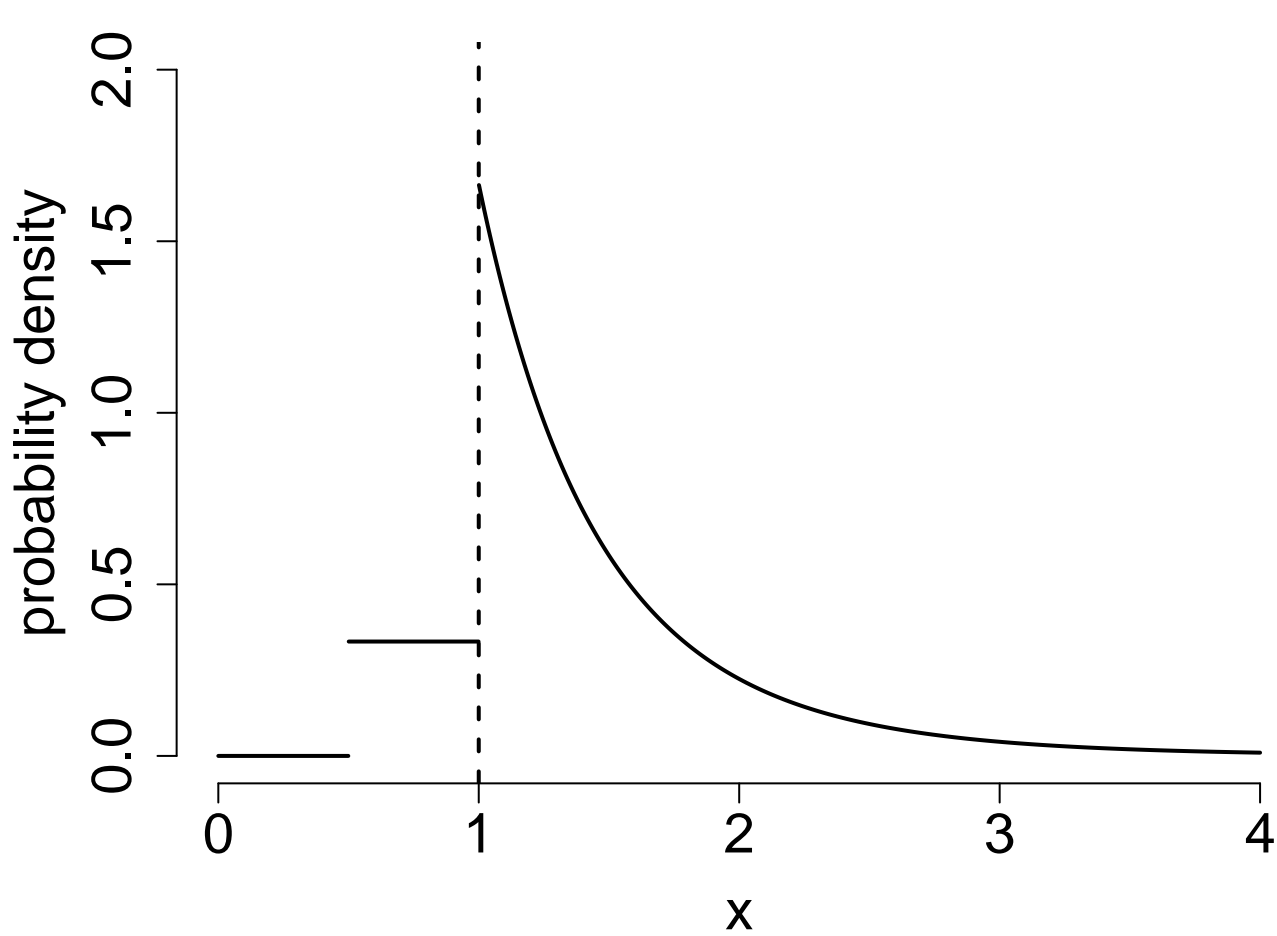

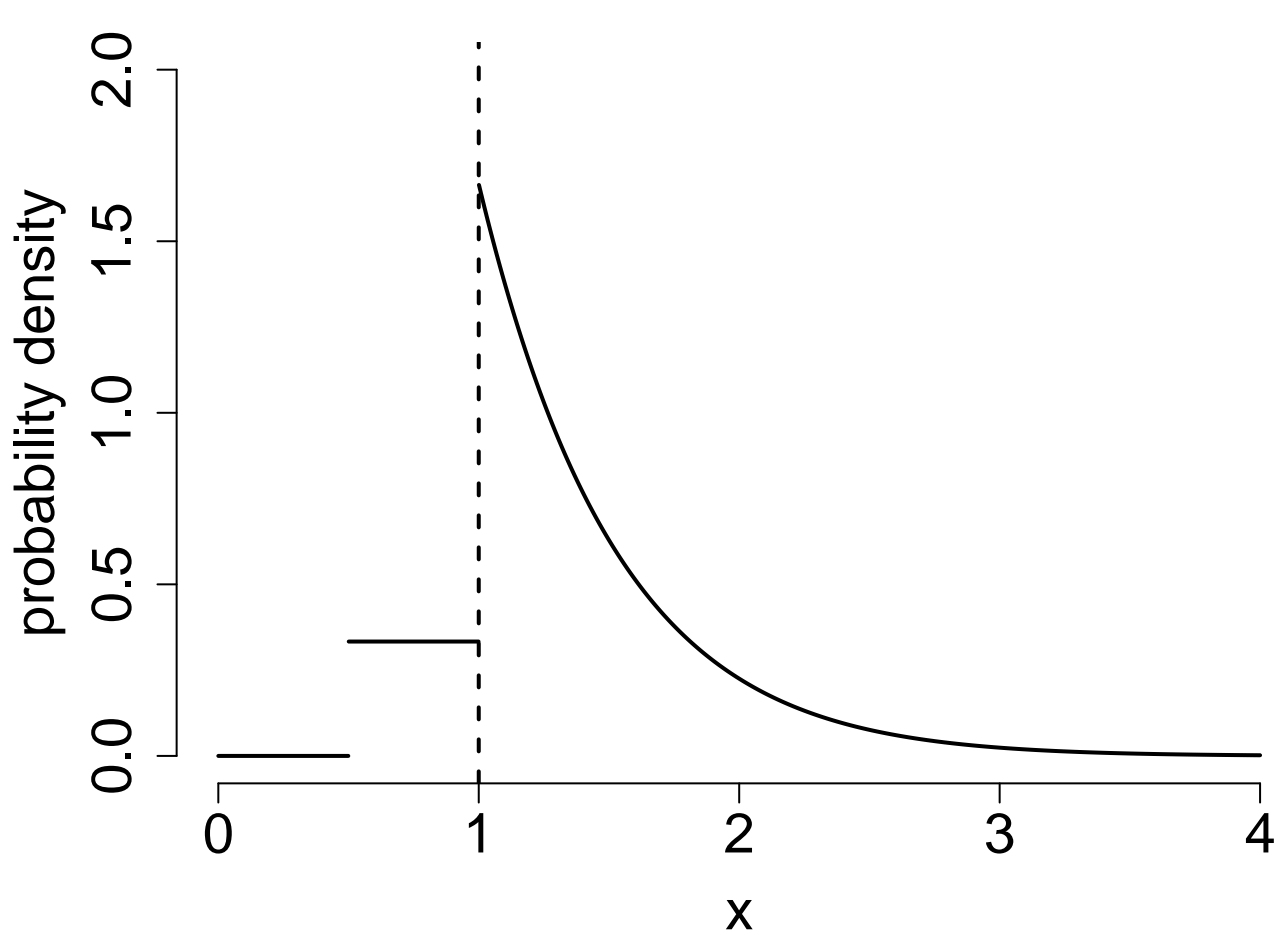

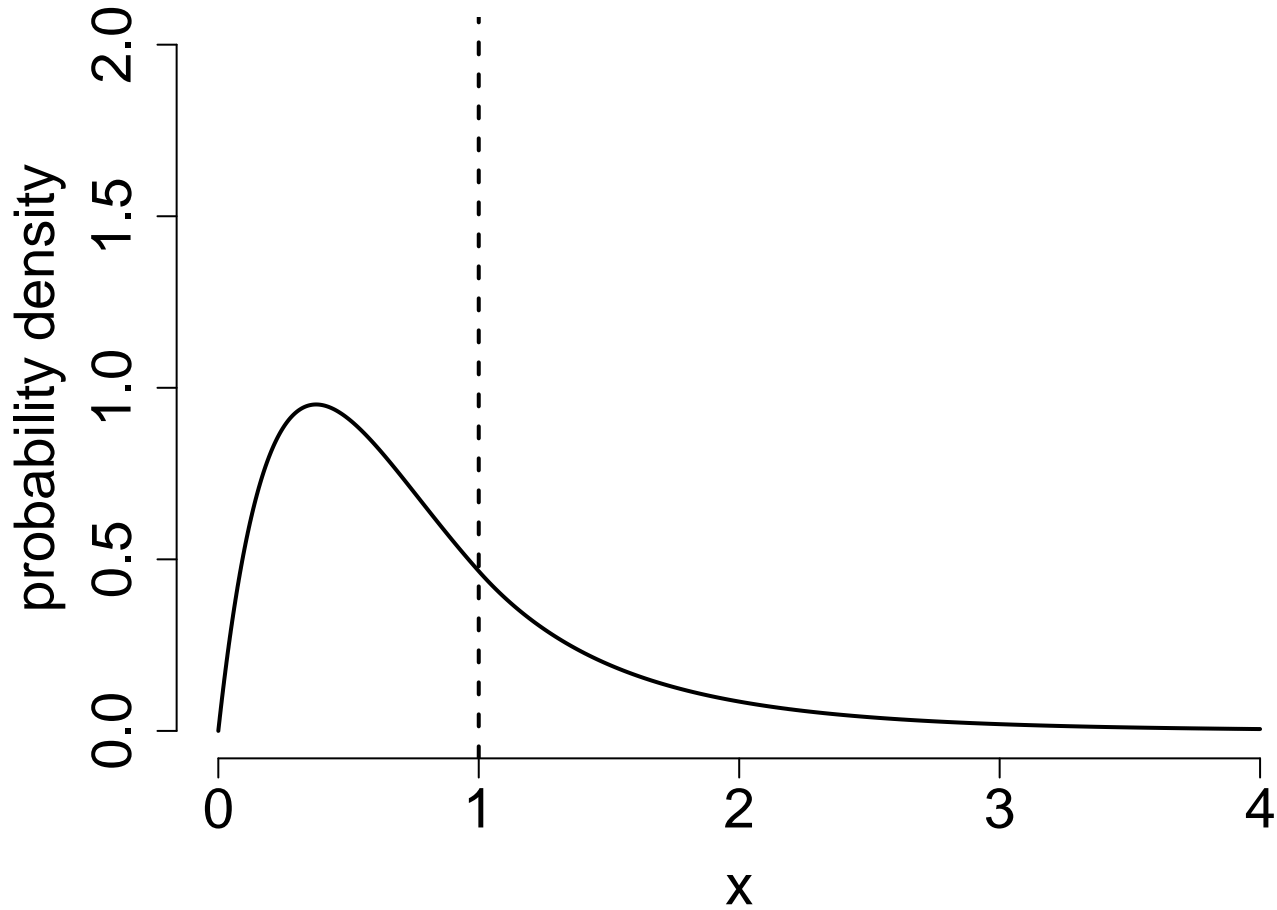

Supplement: Supplementary file 1 [file case_study_denisty_plots.pdf]
